# Supplementary material for: Credible Decentralized Exchange Design via Verifiable Sequencing Rules
Source: arXiv:2209.15569 source file (2023-04-17)
Supplement: Supplementary file 1 [file 9-appendix.tex]

\documentclass[class=article, crop=false]{standalone}

\usepackage{preample}

\begin{document}
\section{Mathematical Background}\label{app:math}
\subimport{./}{10-math-background.tex}

\section{Proof of Pricing Lemma}\label{app:pricing}
\subimport{./}{11-pricing.tex}

\section{Proof of Duality Theorem}\label{app:duality}
\subimport{./}{12-duality.tex}

\end{document}
